# Supplementary material for: ProsaBuddy: Assisting Mechanized Real-Time Schedulability Analysis with LLM-based Agents
Source: arXiv:2610.03796 source file (2026-10-01)
Supplement: Supplementary file 1 [file appendix.tex]

\section*{Appendix}

\subsection{Decomposition}

\begin{itemize}
\item "Proof planner" is a checking script: input: (1) DAG-represented "proof plan" generated by LLM, 
each node is a "proof region", proof region is defined as: 

(2) a .v file generated according to this proof plan DAG:

\item first generate DAG, check: whether it is a valid DAG, not a trivial DAG (only one node)

\item if ok, then next, generate "incomplete proof" 
according to this DAG. check whether this 
"incomplete proof" reflects the DAG.

\item LLM check their consistency, if not, regenerate, ..., 

\item 


\item we want the LLM to generate a "incomplete proof" (a proof with admit) that precisely reflect the proof plan (DAG). 


\item each subagent aims to resolve one of the admit; it works on a copy of the .v file containing the lemma to prove, and we prompt it so that it is not allowed to change any other place, rather than write proofs subsituting the admit. after the subagent finishes, a script will check whether it changes anything else, if yes, then its proof is rejected and this subagent is considered to be failed


\end{itemize}


\subsection{decomposition}

\ljy{If a decomposition remains only in the primary agent's free-form
reasoning, it cannot serve as a reliable basis for the subsequent
proof process. The system cannot mechanically inspect the exact
subgoals, their dependencies, or how their results are intended to
contribute to the original lemma. Consequently, an invalid
decomposition may not be discovered until subagents have attempted
underspecified or unusable subgoals, or until the primary agent fails
to combine their results. ProsaBuddy therefore requires the primary
agent to submit a structured proof plan before constructing the Rocq
proof sketch.

The proof plan is represented as a directed acyclic graph. Each node
records a subgoal stated in Rocq syntax and the predecessor results
that may be used to prove it. A node may also record existing lemmas
that the primary agent proposes to use. Only terminal nodes, i.e.,
nodes that are not further decomposed in the plan, may be marked as
\texttt{delegation\_candidate} and assigned to subagents. The proof
plan thus converts the decomposition from an implicit part of the
LLM's reasoning into an explicit representation on which mechanical
checks can operate.

An explicit plan may still be structurally inconsistent. It may refer
to the wrong target lemma, contain invalid references between nodes,
or introduce circular dependencies for which no subgoal can be proved
first. Before the proof sketch is constructed, ProsaBuddy therefore
checks that the submitted plan matches the target lemma and defines a
well-formed, acyclic dependency structure. These checks reject plans
that cannot provide a consistent order and structure for subsequent
proof construction.

A structurally valid plan may nevertheless rely on an unsuitable
library lemma. In Prosa, a lemma that appears relevant may not be
applicable under the assumptions of the current task model, because
reusable lemmas often require many specific parameters and
preconditions. If these requirements are overlooked, the intended
proof of a subgoal cannot proceed, and the missing premises may become
apparent only after a subagent has started proof search. For a
candidate lemma intended for direct application, ProsaBuddy therefore
uses Rocq to check whether the lemma is applicable in the current
context and whether its remaining premises are available or
represented by predecessor nodes. This check does not prove the
subgoal; it only rules out a planned proof step that is unsupported by
the selected library lemma.

Even a plan that passes these checks is still an abstract description
rather than a Rocq proof. A well-formed graph does not guarantee that
its subgoals are well-typed in their exact local contexts or that their
results can be combined into the original lemma. ProsaBuddy therefore
materializes the accepted plan as a Rocq proof sketch. Each terminal
node selected for delegation is represented by a proof region
containing an \texttt{admit} placeholder, while the proof commands
outside the regions combine the named subgoal results. Compiling this
sketch checks that the subgoal statements are well-typed and that,
assuming the delegated subgoals, the surrounding proof commands close
the original goal.

Because the proof regions still contain \texttt{admit}, this
compilation provides only a conditional guarantee. It can reject a
decomposition whose subgoals cannot be combined into the original
lemma, but it cannot determine whether the individual subgoals are
provable or whether they constitute useful proof progress. 

A delegated subgoal is not extracted from the target proof and stated
as a separate global lemma. Since the subgoal may depend on local
variables, hypotheses, and intermediate results available only at its
position in the original proof, ProsaBuddy asks the subagent to
complete the corresponding proof block in place. This preserves the
exact local context and allows the resulting proof to be used directly
by the surrounding proof commands. However, it also means that the
assigned task appears as one of several local \texttt{admit}
placeholders inside a potentially large and evolving proof. ProsaBuddy
therefore cannot simply ask a subagent to prove the $i$-th
\texttt{admit}: similar placeholders may be difficult for the LLM to
distinguish, and their number and positions may change as the primary
agent refines the decomposition or advances the proof.
To identify these local proof obligations reliably, ProsaBuddy
represents each delegated terminal subgoal as a
\texttt{proof\_region} delimited by annotations written as Rocq
comments. The annotations assign the region a unique identifier and
record its corresponding plan node, target subgoal, and dependencies,
allowing the assigned task to be identified without relying on the
current position of an \texttt{admit}. The region markers also define
the subagent's editable boundary: although the subagent works inside
the original target proof, it may modify only the Rocq source enclosed
by its assigned region. After the subagent returns, ProsaBuddy checks
that the region markers and target subgoal remain unchanged and that
no source outside the region has been modified. An edit that violates
this boundary is rejected and returned to the primary agent for
further handling.
}

\subsection{Watchdog and Progress Evaluator}

\ljy{\textbf{Watchdog and Progress Evaluator.}
The Rocq compiler reports whether the current proof succeeds and, if
not, where it first fails. However, each compiler result describes
only the current proof state; it does not determine whether a sequence
of agent actions is advancing the proof or repeatedly reproducing the
same failure. Consequently, an agent may continue calling the same
tools, launching subagents for an unchanged proof region, or making
superficial edits without recognizing that its current strategy has
stalled. Without an independent assessment of progress, ProsaBuddy
cannot reliably distinguish productive debugging from ineffective
repetition or decide when the agent should revise its current proof
attempt. Such repetition can consume the available computation and
token budget and may prevent the agent from addressing the
decomposition or missing premise that actually blocks the proof.

To address this problem, we develop a Watchdog tool that evaluates
progress during proof construction. We call a point at which the
current proof should be evaluated a \emph{proof milestone}, such as
after the primary agent writes or substantively revises a proof
sketch, after a proof region is updated, or after a subagent returns.
At each milestone, the Watchdog invokes the Rocq compiler and compares
the resulting proof state with the previously recorded state. It
records verified proof progress when Rocq validates a new proof region
or accepts the complete target proof. It also records structural
progress when a proposed decomposition has been materialized as a
well-formed proof sketch, and diagnostic progress when, for example,
the first compiler error moves to a later position in the file. These
forms of progress have different meanings: diagnostic progress shows
that the current attempt has changed the compiler-observed proof state,
but only verified proof progress establishes that an additional
subgoal has been proved. Repeating the same compiler result or making
changes only to comments, identifiers, or whitespace is not considered
progress.

The Progress Evaluator uses the records produced by the Watchdog to
detect stagnation across agent actions. If repeated tool calls or
subagent attempts on the same unchanged proof region produce neither
a newly validated result nor new structural or diagnostic progress,
the Progress Evaluator first warns the agent and may subsequently
prevent another subagent attempt for that region. This restriction is
temporary: another attempt is permitted after the Watchdog observes
new compiler evidence or after the region's subgoal, dependencies, or
proof commands have been substantively revised. The Watchdog and
Progress Evaluator do not establish proof correctness or replace Rocq
and the Validator. Their purpose is to identify when iterative proof
search has stopped producing new evidence and to prevent the agent
from repeatedly consuming computation and tokens without addressing
the cause of the failure.}
