# Supplementary material for: ProsaBuddy: Assisting Mechanized Real-Time Schedulability Analysis with LLM-based Agents
Source: arXiv:2610.03796 source file (2026-10-01)
Supplement: Supplementary file 2 [file supplementary.tex]

\section{Supplementary Material}
Data aggregation, by folder


% This version uses \path{}, so url or hyperref should be loaded.
\onecolumn
{\footnotesize
\setlength{\tabcolsep}{3pt}
\renewcommand{\arraystretch}{0.95}

\begin{longtable}{|c|p{6.1cm}|p{5.3cm}|}
\caption{Training data in Prosa}
\label{tab:benchmark-mapping} \\
\hline
Level & File & Theorem Name \\
\hline
\endfirsthead

\multicolumn{3}{c}{\tablename\ \thetable\ (continued)} \\
\hline
Level & File & Theorem Name \\
\hline
\endhead

\hline
\multicolumn{3}{r}{Continued on next page} \\
\endfoot

\hline
\endlastfoot
level & PROSA file & Statement name \\
\hline
 1 & \path{prosa/analysis/abstract/abstract_rta.v} & \path{job_is_completed_by_arrival_plus_R} \\
\hline
 1 & \path{prosa/analysis/facts/behavior/supply.v} & \path{supply_during_complement} \\
\hline
 1 & \path{prosa/implementation/facts/generic_schedule.v} & \path{schedule_up_to_prefix_inclusion} \\
\hline
 1 & \path{prosa/model/priority/numeric_fixed_priority.v} & \path{NFPD_is_total} \\
\hline
 1 & \path{prosa/results/optimality/edf.v} & \path{EDF_WC_optimality} \\
\hline
 1 & \path{prosa/classic/analysis/apa/bertogna_edf_comp.v} & \path{bertogna_edf_comp_iteration_monotonic} \\
\hline
 1 & \path{prosa/classic/model/arrival/jitter/arrival_sequence.v} & \path{arrived_between_implies_in_actual_arrivals} \\
\hline
 1 & \path{prosa/classic/model/schedule/uni/jitter/schedule.v} & \path{service_before_jitter_is_zero} \\
\hline
 1 & \path{prosa/classic/util/div_mod.v} & \path{modnSor'} \\
\hline
 1 & \path{prosa/classic/analysis/global/basic/bertogna_edf_comp.v} & \path{edf_claimed_bounds_ge_cost} \\
\hline
2 & \path{prosa/analysis/abstract/IBF/task.v} & \path{interference_plus_sched_le_serv_of_task_plus_task_interference_job} \\
\hline
2 & \path{prosa/results/rta/ideal/fp/bounded_pi.v} & \path{A_is_in_concrete_search_space} \\
\hline
2 & \path{prosa/results/transfer_schedulability/criterion.v} & \path{slackless_interval_step_case_completed_job} \\
\hline
2 & \path{prosa/util/nondecreasing.v} & \path{nondecreasing_sequence_undup} \\
\hline
2 & \path{prosa/analysis/abstract/restricted_supply/bounded_bi/jlfp.v} & \path{job_arrival_is_bounded} \\
\hline
2 & \path{prosa/classic/analysis/apa/bertogna_edf_comp.v} & \path{taskset_schedulable_by_edf_rta} \\
\hline
2 & \path{prosa/classic/model/schedule/apa/constrained_deadlines.v} & \path{platform_fp_no_multiple_jobs_of_interfering_tasks} \\
\hline
2 & \path{prosa/util/div_mod.v} & \path{div_ceil_subadditive} \\
\hline
2 & \path{prosa/classic/implementation/apa/schedule.v} & \path{scheduler_apa_work_conserving} \\
\hline
2 & \path{prosa/classic/analysis/global/parallel/workload_bound.v} & \path{workload_bound_n_k_covers_all_jobs} \\
\hline
3 & \path{prosa/analysis/abstract/restricted_supply/abstract_rta.v} & \path{IBF_NP_bounds_interference} \\
\hline
3 & \path{prosa/analysis/facts/model/sbf/periodic.v} & \path{prm_sbf_valid_aux_2} \\
\hline
3 & \path{prosa/rt-proofs-v0.6/implementation/refinements/fast_search_space_computation.v} & \path{task_search_space_subset} \\
\hline
3 & \path{prosa/results/rta/arm/fp/limited_preemptive.v} & \path{uniprocessor_response_time_bound_limited_fp} \\
\hline
3 & \path{prosa/util/nondecreasing.v} & \path{distances_iota_filtered} \\
\hline
3 & \path{prosa/classic/analysis/apa/bertogna_edf_theory.v} & \path{bertogna_edf_interference_by_different_tasks} \\
\hline
3 & \path{prosa/classic/analysis/global/jitter/workload_bound.v} & \path{workload_bound_n_k_covers_middle_jobs} \\
\hline
3 & \path{prosa/classic/implementation/global/basic/schedule.v} & \path{scheduler_completed_jobs_dont_execute} \\
\hline
3 & \path{prosa/classic/model/schedule/uni/limited/fixed_priority/response_time_bound.v} & \path{instantiated_task_interference_is_bounded} \\
\hline
3 & \path{prosa/util/nondecreasing.v} & \path{distance_between_neighboring_elements_le_max_distance_in_seq} \\
\hline
4 & \path{prosa/analysis/abstract/restricted_supply/bounded_bi/edf.v} & \path{longest_bi_with_pi_bound_is_valid} \\
\hline
4 & \path{prosa/results/rta/ovh/edf/limited_preemptive.v} & \path{uniprocessor_response_time_bound_limited_edf} \\
\hline
4 & \path{prosa/util/nondecreasing.v} & \path{max_distance_in_nontrivial_seq_is_positive} \\
\hline
4 & \path{prosa/analysis/facts/busy_interval/existence.v} & \path{busy_interval_is_bounded} \\
\hline
4 & \path{prosa/results/rta/ovh/fp/limited_preemptive.v} & \path{uniprocessor_response_time_bound_limited_fp} \\
\hline
4 & \path{prosa/classic/analysis/apa/bertogna_edf_theory.v} & \path{bertogna_edf_all_cpus_in_affinity_busy} \\
\hline
4 & \path{prosa/classic/analysis/global/jitter/bertogna_fp_theory.v} & \path{bertogna_fp_interference_by_different_tasks} \\
\hline
4 & \path{prosa/classic/analysis/uni/susp/sustainability/singlecost/reduction_properties.v} & \path{sched_susp_highercost_depends_only_on_prefix} \\
\hline
4 & \path{prosa/classic/model/schedule/uni/limited/edf/nonpr_reg/response_time_bound.v} & \path{priority_inversion_is_bounded} \\
\hline
4 & \path{prosa/util/nondecreasing.v} & \path{max_distance_in_nontrivial_seq_is_positive} \\
\hline
5 & \path{prosa/analysis/abstract/restricted_supply/iw_readiness.v} & \path{pending_hep_job_exists_inside_busy_interval} \\
\hline
5 & \path{prosa/analysis/facts/busy_interval/existence.v} & \path{pending_hp_job_exists} \\
\hline
5 & \path{prosa/implementation/refinements/EDF/fast_search_space.v} & \path{search_space_subset_EDF} \\
\hline
5 & \path{prosa/classic/analysis/apa/bertogna_fp_comp.v} & \path{fp_analysis_yields_response_time_bounds} \\
\hline
5 & \path{prosa/classic/analysis/global/basic/bertogna_fp_comp.v} & \path{fp_analysis_yields_response_time_bounds} \\
\hline
5 & \path{prosa/classic/analysis/uni/susp/sustainability/allcosts/reduction_properties.v} & \path{sched_new_work_conserving} \\
\hline
5 & \path{prosa/classic/implementation/apa/schedule.v} & \path{scheduler_priority} \\
\hline
5 & \path{prosa/classic/model/schedule/global/jitter/platform.v} & \path{work_conserving_eq_work_conserving_count} \\
\hline
5 & \path{prosa/classic/model/schedule/uni/limited/fixed_priority/nonpr_reg/concrete_models/response_time_bound.v} & \path{uniprocessor_response_time_bound_fp_with_floating_nonpreemptive_regions} \\
\hline
5 & \path{prosa/classic/analysis/global/parallel/bertogna_fp_comp.v} & \path{fp_analysis_yields_response_time_bounds} \\
\hline
6 & \path{prosa/classic/analysis/apa/bertogna_edf_comp.v} & \path{bertogna_edf_comp_rt_grows_too_much} \\
\hline
6 & \path{prosa/classic/analysis/global/basic/bertogna_edf_comp.v} & \path{bertogna_edf_comp_rt_grows_too_much} \\
\hline
6 & \path{prosa/classic/analysis/global/jitter/interference_bound_edf.v} & \path{interference_bound_edf_holds_for_single_job_that_completes_on_time} \\
\hline
6 & \path{prosa/classic/analysis/global/parallel/bertogna_edf_theory.v} & \path{bertogna_edf_interference_on_all_cpus} \\
\hline
6 & \path{prosa/classic/analysis/uni/susp/dynamic/jitter/jitter_schedule_service.v} & \path{jitter_reduction_inductive_step_case2} \\
\hline
6 & \path{prosa/classic/model/schedule/uni/limited/abstract_RTA/abstract_rta.v} & \path{job_completed_by_arrival_plus_R_2} \\
\hline
6 & \path{prosa/classic/model/schedule/uni/limited/jlfp_instantiation.v} & \path{instantiated_quiet_time_equivalent_edf_quiet_time} \\
\hline
6 & \path{prosa/classic/model/schedule/uni/limited/platform/priority_inversion_is_bounded.v} & \path{not_quiet_implies_exists_scheduled_hp_job_at_preemption_point} \\
\hline
6 & \path{prosa/classic/model/schedule/uni/susp/build_suspension_table.v} & \path{suspension_duration_matches_predicate_up_to_t_max} \\
\hline
6 & \path{prosa/classic/model/schedule/uni/susp/suspension_intervals.v} & \path{cumulative_suspension_eq_total_suspension} \\
\hline
7 & \path{prosa/classic/analysis/apa/bertogna_fp_theory.v} & \path{bertogna_fp_interference_in_non_full_processors} \\
\hline
7 & \path{prosa/classic/analysis/global/parallel/bertogna_edf_comp.v} & \path{bertogna_edf_comp_iteration_preserves_order} \\
\hline
7 & \path{prosa/classic/analysis/uni/basic/tdma_wcrt_analysis.v} & \path{formula_sched_St} \\
\hline
7 & \path{prosa/classic/model/schedule/uni/limited/abstract_RTA/abstract_seq_rta.v} & \path{bound_for_cumulative_job_interference_actual} \\
\hline
7 & \path{prosa/classic/model/schedule/uni/limited/platform/priority_inversion_is_bounded.v} & \path{preemption_time_exists} \\
\hline

\end{longtable}
}

\twocolumn



% 如果你的论文是双栏，并且这张表要跨页，最稳的是临时切成单栏
\onecolumn
{\footnotesize
\setlength{\tabcolsep}{3pt}
\renewcommand{\arraystretch}{0.95}

\begin{longtable}{|c|p{6.1cm}|p{5.3cm}|}
\caption{Test data in Prosa}
\label{tab:benchmark-mapping} \\
\hline
Level & File & Theorem Name \\
\hline
\endfirsthead

\multicolumn{3}{c}{\tablename\ \thetable\ (continued)} \\
\hline
Level & File & Theorem Name \\
\hline
\endhead

\hline
\multicolumn{3}{r}{Continued on next page} \\
\endfoot

\hline
\endlastfoot
1 & \path{prosa/analysis/abstract/abstract_rta.v} & \path{uniprocessor_response_time_bound} \\
\hline
1 & \path{prosa/analysis/facts/behavior/arrivals.v} & \path{any_ready_job_is_pending} \\
\hline
1 & \path{prosa/model/task/arrival/sporadic_as_curve.v} & \path{sporadic_arrival_curve_valid} \\
\hline
1 & \path{prosa/implementation/refinements/EDF/fast_search_space.v} & \path{EDF_ss_generalize_FP_ss} \\
\hline
1 & \path{prosa/results/transfer_schedulability/criterion.v} & \path{ref_transfer_schedulability_criterion_sufficiency} \\
\hline
1 & \path{prosa/classic/analysis/global/parallel/bertogna_edf_theory.v} & \path{bertogna_edf_specific_bound_holds} \\
\hline
1 & \path{prosa/classic/analysis/uni/basic/fp_rta_comp.v} & \path{taskset_schedulable_by_fp_rta} \\
\hline
1 & \path{prosa/classic/model/arrival/basic/arrival_bounds.v} & \path{sporadic_task_arrival_bound} \\
\hline
1 & \path{prosa/classic/implementation/apa/schedule.v} & \path{scheduler_mapping_respects_affinity} \\
\hline
1 & \path{prosa/classic/util/minmax.v} & \path{seq_max_nat_computes_max} \\
\hline
2 & \path{prosa/analysis/abstract/busy_interval.v} & \path{busy_interval_has_uninterrupted_service} \\
\hline
2 & \path{prosa/analysis/abstract/IBF/task.v} & \path{task_IBF_implies_job_IBF} \\
\hline
2 & \path{prosa/analysis/abstract/restricted_supply/search_space/fifo_fixpoint.v} & \path{soln_abstract_response_time_recurrence} \\
\hline
2 & \path{prosa/implementation/refinements/fast_search_space_computation.v} & \path{multiple_of_horizon_in_approx_ss} \\
\hline
2 & \path{prosa/results/transfer_schedulability/criterion.v} & \path{slackless_interval_existence} \\
\hline
2 & \path{prosa/classic/analysis/apa/bertogna_edf_theory.v} & \path{bertogna_cirinei_response_time_bound_edf} \\
\hline
2 & \path{prosa/classic/analysis/global/jitter/bertogna_edf_theory.v} & \path{bertogna_edf_workload_bounds_interference} \\
\hline
2 & \path{prosa/classic/analysis/uni/basic/tdma_wcrt_analysis.v} & \path{exists_WCRT} \\
\hline
2 & \path{prosa/classic/analysis/uni/susp/dynamic/oblivious/fp_rta.v} & \path{suspension_oblivious_fp_rta_implies_schedulability} \\
\hline
2 & \path{prosa/classic/model/schedule/global/transformation/construction.v} & \path{service_dependent_schedule_construction} \\
\hline
3 & \path{prosa/analysis/abstract/busy_interval.v} & \path{busy_interval_is_bounded} \\
\hline
3 & \path{prosa/analysis/facts/behavior/arrivals.v} & \path{arrivals_between_sorted} \\
\hline
3 & \path{prosa/implementation/refinements/EDF/nonpreemptive_sched.v} & \path{sched_nonpreemptive_next} \\
\hline
3 & \path{prosa/results/rta/ideal/elf/bounded_pi.v} & \path{instantiated_busy_intervals_are_bounded} \\
\hline
3 & \path{prosa/util/search_arg.v} & \path{search_arg_extremum} \\
\hline
3 & \path{prosa/classic/analysis/apa/bertogna_fp_theory.v} & \path{bertogna_fp_workload_bounds_interference} \\
\hline
3 & \path{prosa/classic/analysis/global/parallel/interference_bound_edf.v} & \path{interference_bound_edf_n_k_covers_all_jobs} \\
\hline
3 & \path{prosa/classic/analysis/uni/basic/fp_rta_theory.v} & \path{uniprocessor_response_time_bound_fp} \\
\hline
3 & \path{prosa/classic/implementation/apa/schedule.v} & \path{scheduler_mapping_is_work_conserving} \\
\hline
3 & \path{prosa/classic/model/schedule/uni/limited/abstract_RTA/reduction_of_search_space.v} & \path{representative_exists} \\
\hline
4 & \path{prosa/analysis/abstract/ideal/iw_instantiation.v} & \path{quiet_time_ab_implies_quiet_time_cl} \\
\hline
4 & \path{prosa/analysis/facts/behavior/service.v} & \path{incremental_service_during} \\
\hline
4 & \path{prosa/analysis/facts/model/overheads/blackout_bound.v} & \path{fin_sched_changes_start_busy_pref_bounded_overheads_blackout} \\
\hline
4 & \path{prosa/results/rta/ovh/edf/fully_nonpreemptive.v} & \path{uniprocessor_response_time_bound_fully_nonpreemptive_edf} \\
\hline
4 & \path{prosa/util/unit_growth.v} & \path{slowed_subtraction_value_preservation} \\
\hline
4 & \path{prosa/classic/analysis/apa/bertogna_edf_comp.v} & \path{bertogna_edf_comp_f_increases} \\
\hline
4 & \path{prosa/classic/analysis/apa/bertogna_fp_theory.v} & \path{bertogna_fp_all_cpus_in_subaffinity_busy} \\
\hline
4 & \path{prosa/classic/analysis/uni/basic/tdma_wcrt_analysis.v} & \path{formula_not_sched_St} \\
\hline
4 & \path{prosa/classic/model/schedule/global/basic/constrained_deadlines.v} & \path{platform_cpus_busy_with_interfering_tasks} \\
\hline
4 & \path{prosa/classic/util/div_mod.v} & \path{divSn_cases} \\
\hline
5 & \path{prosa/classic/analysis/apa/bertogna_edf_comp.v} & \path{edf_claimed_bounds_finds_fixed_point_of_list} \\
\hline
5 & \path{prosa/classic/analysis/global/basic/bertogna_edf_comp.v} & \path{edf_claimed_bounds_finds_fixed_point_of_list} \\
\hline
5 & \path{prosa/classic/analysis/global/basic/interference_bound_edf.v} & \path{interference_bound_edf_holds_for_single_job_that_completes_on_time} \\
\hline
5 & \path{prosa/classic/analysis/global/jitter/bertogna_edf_comp.v} & \path{edf_claimed_bounds_finds_fixed_point_of_list} \\
\hline
5 & \path{prosa/classic/analysis/global/jitter/bertogna_fp_comp.v} & \path{fp_analysis_yields_response_time_bounds} \\
\hline
5 & \path{prosa/classic/analysis/global/parallel/bertogna_edf_comp.v} & \path{edf_claimed_bounds_finds_fixed_point_of_list} \\
\hline
5 & \path{prosa/classic/analysis/uni/basic/tdma_wcrt_analysis.v} & \path{response_time_le_WCRT} \\
\hline
5 & \path{prosa/classic/analysis/uni/susp/dynamic/jitter/jitter_schedule_properties.v} & \path{sched_jitter_respects_policy} \\
\hline
5 & \path{prosa/classic/model/schedule/uni/limited/abstract_RTA/abstract_seq_rta.v} & \path{task_rbf_excl_tsk_bounds_task_workload_excl_j} \\
\hline
5 & \path{prosa/classic/model/schedule/uni/limited/edf/nonpr_reg/concrete_models/response_time_bound.v} & \path{uniprocessor_response_time_bound_edf_with_floating_nonpreemptive_regions} \\
\hline
6 & \path{prosa/classic/analysis/apa/bertogna_edf_theory.v} & \path{bertogna_edf_alpha'_is_full} \\
\hline
6 & \path{prosa/classic/analysis/global/basic/bertogna_edf_theory.v} & \path{bertogna_edf_interference_in_non_full_processors} \\
\hline
6 & \path{prosa/classic/analysis/global/jitter/bertogna_edf_comp.v} & \path{bertogna_edf_comp_rt_grows_too_much} \\
\hline
6 & \path{prosa/classic/analysis/global/parallel/bertogna_edf_comp.v} & \path{bertogna_edf_comp_rt_grows_too_much} \\
\hline
6 & \path{prosa/classic/analysis/global/parallel/bertogna_fp_theory.v} & \path{bertogna_fp_all_cpus_are_busy} \\
\hline
6 & \path{prosa/classic/model/schedule/uni/limited/busy_interval.v} & \path{busy_interval_is_bounded} \\
\hline
6 & \path{prosa/classic/model/schedule/uni/limited/busy_interval.v} & \path{pending_hp_job_exists} \\
\hline
6 & \path{prosa/classic/model/schedule/uni/limited/edf/response_time_bound.v} & \path{A_is_in_concrete_search_space} \\
\hline
6 & \path{prosa/classic/model/schedule/uni/limited/jlfp_instantiation.v} & \path{instantiated_cumulative_interference_of_hep_jobs_equal_total_interference_of_hep_jobs} \\
\hline
6 & \path{prosa/classic/model/schedule/uni/service.v} & \path{incremental_service_during} \\
\hline
7 & \path{prosa/classic/analysis/apa/bertogna_edf_comp.v} & \path{bertogna_edf_comp_iteration_preserves_order} \\
\hline
7 & \path{prosa/classic/analysis/global/jitter/bertogna_edf_comp.v} & \path{bertogna_edf_comp_iteration_preserves_order} \\
\hline
7 & \path{prosa/classic/analysis/global/basic/bertogna_edf_comp.v} & \path{bertogna_edf_comp_iteration_preserves_order} \\
\hline
7 & \path{prosa/classic/model/schedule/uni/limited/fixed_priority/nonpr_reg/concrete_models/response_time_bound.v} & \path{uniprocessor_response_time_bound_fp_with_fixed_preemption_points} \\
\hline
7 & \path{prosa/classic/model/schedule/uni/limited/edf/nonpr_reg/concrete_models/response_time_bound.v} & \path{uniprocessor_response_time_bound_edf_with_fixed_preemption_points} \\
\hline

\end{longtable}
}

\twocolumn

1. Case study model folder     get
\begin{itemize}
    \item Number of Data Items: 24
    \item Data File Structure: \begin{itemize}
        \item a. Modeling files (.v files)
        \item b. Related paper files (.pdf files)
        \item c. Detailed proofs of theorems from the papers (.tex files)
        \item d. A small number of data has images from the papers that the proofs depend on (.png files)
    \end{itemize}
\end{itemize}

2. Prosabuddy for casestudy  get

Problem of data: \begin{itemize}
\item  case1 finished but state shows Proof verified: no
\item case3 is not the success one,but have on influence on results
\item  lack of case 5,6,7
\item case8 is not the results in table
\item case9 is  not the results in table
\item lack of case 11
\item case14 is  not the results in table
\item case15 rerun
\item lack of case 22,23
\item case10,13,19 prompt are different, no paper



\end{itemize}

3. PALM for casestudy  get
\begin{itemize}
    \item Number of Data Items:9
\end{itemize}
Problem
\begin{itemize}
    \item Missing 15 cases2,3,4,8,9,12-18,20,21,23
     \item no run 3,15,16,18,20,21,23
    \item without the result .v
\end{itemize}

4. Rocqstar for casestudy  get

\begin{itemize}
    \item Number of Data Items:13
\end{itemize}
Problem
\begin{itemize}
    \item Missing 11 cases2,3,4,5,8,9,15,16,17,18,23
    \item no run 3,15,16,18,20,21,23
    \item without the result .v
\end{itemize}



5. Copra for casestudy  get
\begin{itemize}
    \item Number of Data Items:10
\end{itemize}
Problem:
\begin{itemize}
    \item Missing 14 cases2,3,4,8,9,12,14-18,20,21,23
     \item no run 3,15,16,18,20,21,23
    \item without the result .v
    \item without result in table
\end{itemize}


6. Opencode for casestudy get complete

  





7. PB-w/o-skill and decompose for casestudy complete
\begin{itemize}

    \item no data for this setting
\end{itemize}

8. PB-w/o-skill for casestudy   get
\begin{itemize}
    \item Number of Data Items:19
\end{itemize}
Problem:
\begin{itemize}
    \item Missing 5 cases9,16,20,21,24
    \item no run, 16,20,21
    \item Important !!!! case 16 in the table are $\infty$ but no data
    
    \ljy{
    \item case12 is $\infty$ or success, allow to add head files?(need to delete one)
    \item case8 has same problem}
    
    \item case23 need new results

\end{itemize}

9. PB-w/o-decompose for casestudy    get 

\begin{itemize}
    \item Number of Data Items: 4,case 2,4,9,14,
    
\end{itemize}
Problem:
\begin{itemize}
    \item Missing 20 cases
    \item Important !!!! case1,5,6,7,10,11,12,13,17,19,22,23,24in the table are success but no data
    \item no run 15,16,18,20,21,23
    \item Important !!! The prompts in all data instruct to split, which does not match the experimental setting. not use subagent but decompose
    \item prompt difference:Difference in Readable Scope:
this version strictly limits the readable scope to the target file, proof.tex, and prosa . other version allows reading any directly relevant content within the current workspace 

Difference in Reusable Proof Artifacts:
this version only permits the reuse of the target .v file and Prosa . Other version extends this to include any directly relevant proof artifacts within the workspace .

    \item Important!!! case14 token is 24499K, The process stopped due to an unknown external interruption, leading to an incorrect label in the table. It needs to be rerun.
\end{itemize}


10. PB-w/o-hint for casestudy    get
\begin{itemize}
    \item Number of Data Items: 17,case 1,2,3,4,5,6,7,9,10,11,12,13,17,19,20,22,24
\end{itemize}

\begin{itemize}
    \item Missing 7 cases : 8,14,15,16,18,21,23
    \item no run 15,16,18,21,23
    \item The prompt didn't restrict reading papers; instead, it instructed to read the paper first if available. It's just that there were no papers provided in the workspace for it to read.
    
\end{itemize}


11. PB-w/o-prosa for casestudy     get
\begin{itemize}
    \item Number of Data Items: 15,case 1,2,3,4,5,6,7,9,10,11,12,13,19,22,24
\end{itemize}

Problem:
\begin{itemize}
    \item Missing 9cases : 8,14,15,16,17,18,20,21,23
    \item     no run 15,16,18,20,21,23
    \item Important !!!! case 17in the table are success but no data
    \item case22 should be $\infty$
\end{itemize}


12.PB-with-deepseekv4flash for casestudy    get  complete

\begin{itemize}
    \item Number of Data Items:24case 
\end{itemize}






13. PB-with-deepseekv4pro for casestudy get complete
\begin{itemize}
    \item Number of Data Items: 19,case
    \end{itemize}
  Problem: 
 
  \begin{itemize}

    \item  5cases no run : 15,16,18,20,21



  

\end{itemize}



14. PB-with-Gemini for casestudy get
\begin{itemize}
    \item Number of Data Items: 6,case 5,6,10,11,19,23
    \end{itemize}
  Problem: 
  \begin{itemize}
    \item Missing 18cases
    \item  6cases no run : 3,15,16,18,20,21
    \item need 12 cases : 1,2,4,7,8,9,12,13,14,17,22, 24
 
    \item case10,11 is x wrong in table


\end{itemize}





15. PB-with-QWen for casestudy get
\begin{itemize}
    \item Number of Data Items: 17
    \end{itemize}
  Problem: 
  \begin{itemize}
    \item Missing 7cases 
    \item case 23 is wrong ,need to rerun
    \item many case failed by timeout, only about 5M token

\end{itemize}

16.Dataset for prosa get complete

17. Prosabuddy for prosa get
\begin{itemize}
    \item level1 :running

    \item  level2 :9/10 miss data 1 
    
    \item level3 : complete

    \item level4 9/10 miss data 1
    \item level5 8/10 miss data 1,7
    \item level6 9/10 miss data 1 results are very different with table 
    \end{itemize}



18.PALM for prosa get
\begin{itemize}
    \item level 1 1/10 complete
    \item no results for level2 and 3
\end{itemize}

19.Rocqstar for prosa  get
\begin{itemize}
    \item level 1 7/10 No.4 no data
      \item no results for level2 and 3
\end{itemize}

20.Copra for prosa get
\begin{itemize}
    \item level 1 0/10 complete
     \item no results for level2 and 3
\end{itemize}

21.Opencode for prosa  get
\begin{itemize}

    \item level 1 4/10 complete
     \item level 2 0/10 complete
     \item level 3 no results
\end{itemize}



\subsection{Submitted Materials}
\begin{itemize}
\item 
\item
\item
\end{itemize}


\subsection{ProsaBuddy - Formalization Assistant}
\guan{implicit assumptions?}

When researcher uses the Prosa approach to prove the lemmas of a research paper, the first significant effort is required to formalize the lemmas in Coq/Rocq, 
i.e., transfer the lemma description in natural language into the formal language in Coq/Rocq.
The lemma we will prove in schedulability analysis builds upon a much more complex foundation of concepts,
including many levels of definitions, assumptions.
The concepts of the pure mathematics problems are typically using much simpler concepts. Figure \ref{} shows a mathematical problem in XXX benchmark as an example and Figure \ref{} shows an example of a real-time schedulability analysis lemma in Prosa. 
Therefore, \ours\ include a \oursformal\ to help the lemma formalization and reduce the user's effort.



The output of \oursformal\ must still go through very careful manual checking by human users. This is because there is no possible automated way to formally verify 
the equivalence between a natrual language statement and its formalized statement due to the inherent ambiguity of natural langauge \cite{??}. The target of \oursformal\ is not to provide a fully automated formalization tool, but instead, only to mitigate the effort of doing some tedious work in the lemma formalization procedure. 





As mentioned in Section \ref{}, the formalization of a lemma in Coq/Rocq consists of three parts: (1) variables, (2) definitions and (3) hypothesis and (4) the lemma statement.


The Formalization Assistant adopts a popular Writer/Reviewer dual agent architecture which is widely used in writing-style tasks:
the writer will write a formalization, then the reviewer reviews it and identify potential problems of the formalization generated by the Writer, and send it back to the Writer to revise it. This process repeats until the reviewer \enquote{approves} the formalization generated by the writer.
Both the Writer and the Reviewer will use external tools \guan{?} as will be detailed later. We instruct the writer and reviewer by giving them different prompts.  
The reason why such a Writer/Reviewer agent architecture is effective is because, it is good to ask the same agent to do two things that \enquote{contradicting} with each other. 



\subsection{The Writer Agent}
The prompt to Writer execute the following steps:
\begin{enumerate}
    

\item Reading materials.
Read the natural-language description relevant to understanding the target lemma: its statement plus all preceding definitions, assumptions, notations, and explanatory paragraphs that define or constrain any object, symbol, or condition used in the target result. 
\guan{also read prosa}

\item Semantic division. 
Break the text into a list of concept blocks, each centered on one primary semantic unit (e.g., an object, relation, assumption, definition). Split composite concepts into their semantic parts and add implicit modeling blocks if needed. For each block, record its source, role, dependencies, introduced symbols, and whether it is directly needed for the theorem statement. 

\item Formalizing each concept block.

Map each concept block to Prosa or local formalization.
Decide for each block whether to reuse an existing Prosa concept, instantiate a Prosa abstraction, or introduce a paper‑local Variable, Definition, or Hypothesis. Reuse Prosa whenever possible. Use Variable for external parameters that the theorem should hold for any legal instance, Definition for uniquely determined derived notions, and Hypothesis for properties or legality conditions. A single paper concept may map to multiple Coq declarations. Every Coq object introduced must correspond to an explicit or justified implicit block.

\item Formalize the model. Write the Coq imports, section structure, Variables, Definitions, and Hypothesises in dependency order (foundational objects first). Add short comments only when the mapping is not obvious. Do not redefine existing Prosa concepts. Ensure that by the end of this step, every symbol and condition needed for the target theorem statement already exists in Coq. Justify any implicit assumption with a brief comment.

\item Write the target theorem/lemma.
State the theorem or lemma exactly as a Coq Theorem or Lemma, using only the concepts already introduced in Steps 3 and 4. The statement must faithfully express the mathematical meaning of the paper’s result. Do not introduce any new Variable, Definition, or Hypothesis here. End the proof with Admitted.

\item Validate the formalization.
Verify that the generated .v file compiles with coqc. Check that every symbol in the theorem statement traces back to an explicit or justified implicit block from before the theorem. Ensure that no material after the target result was used, no Prosa concept was unnecessarily redefined, and any implicit assumptions imported from Prosa are reasonable consequences of the paper’s intended model or of the chosen Prosa abstraction.
\end{enumerate}


\begin{itemize}

\item First read the natural-language description related to the lemma to be formalized. This includes not only the lemma statement itself, but also includes other descriptions about the concepts used.

\item Semantics Decomposition: to divide the informal description to make a list of objects (each object is a text block), which describe an object or assumption that may be needed to state the lemma? mapping

\item Check the Prosa Library to select 
variables, definitions and hypothesis that already exists in Prosa Library that can be used to model the concept described in each block.

\item Formalize the needed variables, definitions and hypothesis that does not exists in Prosa Library.

\item Write the Lemma statement.


\item Check the syntax correctness. If there is syntax error, fix the error and regenerate the entire formalization and check the syntax correctness again, and repeats until it is syntax correct. In our experiments, we found that in case syntax error happens, it typically can be quickly fixed in a few iterations.
\end{itemize}



2. skill:Its main rule is: decompose semantics first, reuse existing PROSA notions whenever possible, use \verb|Variable| only for genuine external inputs \guan{what is this?}, use \verb|Definition| for context-determined meaning, and use \verb|Hypothesis| only for properties of already-defined objects. In short, it is a discipline for making theorem skeletons semantically precise instead of superficially matching paper terminology. 

Important methodological point :
1) A \verb|Variable| should be used only for an externally supplied object that the theorem ranges over for any legal instance, and that cannot be uniquely computed from the current context.
A \verb|Definition| should be used for meanings uniquely determined by the current context, such as formulas, sets, windows, bounds, predicates, classifications, or maxima and minima.
A \verb|Hypothesis| should be used only to state that an already existing object satisfies some property. In other words, define the property as a predicate first, and only then assume or prove that it holds. 

2) \guan{is everything here by prompt?} First check whether a concept is composite; if so, split it into multiple semantic components and handle them separately.
Then check whether PROSA already provides the corresponding notion; if it does, reuse it directly rather than redefining or wrapping it.
Only define a new notion when PROSA does not already provide it and the meaning is uniquely determined by the current context.
Statements about existence, uniqueness, maximality, minimality, or the validity of an upper bound should not be modeled as Definitions; they belong in Lemma, Theorem, or sometimes Hypothesis \guan{why??}.



\guan{should not force it to strictly follow the original text, but should think of potential implicit assumption}


In the prompt, we teach the LLM how to 


\subsection{The Reviewer Agent}





The Reviewer agent checks both the syntax correctness and the semantic correctness of the formalization writing generated by the Writer agent, and approves the formalization writing only if it thinks the formalization is correct in both aspects.


The prompt to Reviewer includes the following key points:
\begin{itemize}
\item PROSA-first review is mandatory. For every paper concept, require direct reuse
    of existing PROSA definitions, foundational model components, generic hypotheses,
    reusable interfaces, and naming conventions whenever suitable PROSA vocabulary
    exists. Treat avoidable redefinitions, aliases, wrappers, or paper-local encodings
    around PROSA-provided concepts as review issues unless the file documents a
    genuine paper-specific refinement over the PROSA primitive.


\item Reconstruct the actual meaning of the important Coq definitions and hypotheses
    in plain language and compare them to the paper semantics. Flag weak, trivial,
    unrelated, or semantically mismatched theorem statements as blocking issues.

\item Decision rule: set decision=approve if and only if $blocking_count==0$ and the
theorem/lemma modeling contract is fully satisfied. Compile failures, missing
target Coq file, missing compile status, forbidden Abort/Axiom, paper semantic
mismatches, unjustified assumptions, use of post-target paper content, or a weak,
trivial, or unrelated target theorem/lemma statement are blocking issues.
\end{itemize}


\subsection{Implementation}

\guan{
\begin{itemize}
\item 
\item
\end{itemize}
}

\guan{my writing ends here !!!!!!!!!!!!!!! }



\guan{ written by junyi }

We design a two-agent formalization workflow for translating real-time systems paper results into Coq/PROSA artifacts. For each benchmark instance, the runner creates an isolated workspace containing the original paper PDF, the local PROSA library, a workspace-local modeling skill, and a machine-readable target specification. The first agent, Agent1, is launched as a persistent opencode session with access to the workspace and the original PDF attachments. Agent1 is instructed to read only the paper content up to the target theorem or lemma, reuse existing PROSA concepts whenever possible, construct a compilable Coq file, record compilation status, and then request review through a dedicated MCP tool \guan{does it mean that agent 1 "call" agent 2 as a MCP tool?}.

The review tool is implemented by a Python MCP server. When Agent1 calls request\_review \guan{what is "request\_review", is it a function or something?}, the server \guan{the MCP server?} invokes a second persistent opencode session, Agent2, in the same workspace. On its first invocation, Agent2 receives the original PDF attachments and a reviewer role prompt; subsequent invocations resume the same session using the stored session identifier, preserving review context across iterations. Agent2 is permission-restricted to read-only behavior: editing, shell execution \guan{why?}, subtask creation, and recursive MCP calls are denied. Its output must be a structured JSON review containing a decision, issue list, coverage checks, formula checks, and semantic reconstructions of the Coq artifacts.

To prevent false approvals \guan{what is false approval}, the system layers a deterministic gate over Agent2’s semantic judgment. The gate checks that the target Coq file, target specification, and compilation report exist; that compilation is reported as passing; that forbidden constructs such as Abort and Axiom are absent; and that the review schema includes the required semantic fields. It also converts uncovered concepts, missing formulas, and semantic mismatches reported by Agent2 into blocking or major issues. The final approval decision is recomputed by the gate: an artifact is accepted only when no blocking issues remain. If the decision is revise, Agent1 updates the formalization, recompiles, and calls the review tool again. If the decision is approve, Agent1 writes a final exit report and the runner records the experiment as approved.

%end rtc added

Design:







\subsection{Result Analysis of Formalization}


Results Analysis:
1. Overly strong semantics (case 6)
paper: Even if we don’t know the location of
this instance, nor the conditions at which it is maximally interfered, we can anyway denote it with \(J_k^*\)

\guan{??\\}

Correct version:
\begin{verbatim} 
Hypothesis j_has_max_interference:
forall j0 , job_task j0=tsk ->arrives_in arr_seq j0 ->
total_interference job_arrival job_cost sched j0 (job_arrival j0) (job_arrival j0+R)
<=total_interference job_arrival job_cost sched j (job_arrival j) (job_arrival j+R). 
\end{verbatim}

Wrong version: 

\begin{verbatim} 
  (* Paper proof notation for Theorem 3: J_k^* is the job that suffers the maximum response time. *)
  Definition is_maximum_response_time_witness (tsk : sporadic_task) (j_star : Job) : Prop :=
    arrives_in arr_seq j_star /\
    job_task j_star = tsk /\
    exists R_star,
      job_response_time_eq j_star R_star /\
      forall j R_j,
        arrives_in arr_seq j ->
        job_task j = tsk ->
        job_response_time_eq j R_j ->
        R_j <= R_star.
\end{verbatim}
The job that suffers the maximum interference in the erroneous version is modeled as the semantically stronger job with the maximum response time.


2. Overly weak semantics (case 9)

paper: We restrict that a job \(J_i^h\)
can execute only if its precedent job \(J_i^{h-1}\) has been already finished, to avoid unnecessary working space conflict.

Correct version:
\begin{verbatim}
  Hypothesis H_sequential_tasks:
      forall j1 j2 t cpu,
        arrives_in arr_seq j1 ->
        arrives_in arr_seq j2 ->
        job_task j1 = job_task j2 ->
        job_arrival j1 < job_arrival j2 ->
        scheduled_on sched j2 cpu t ->
        completed job_cost sched j1 t.
\end{verbatim}

Wrong version: 
{
\tiny
\begin{verbatim}
Hypothesis H_tasks_do_not_execute_in_parallel :
    jobs_of_same_task_dont_execute_in_parallel job_task sched.
\end{verbatim}}
The erroneous version models the condition that a job can only execute after its predecessor job has completed as a task having at most one job running at a time. This results in weaker semantics and loses the part of the original semantics where jobs execute sequentially.

(case 11)
\begin{verbatim}
 Variable busy_end : time.
  
    (* The analyzed job finishes after its release, so the busy window is non-empty. *)
    Hypothesis H_release_before_busy_end :
      job_arrival analyzed_job < busy_end.
\end{verbatim}
The paper explicitly states that the busy period ends at the finish time of $J_k$, whereas this modeling only assumes it ends after the arrival time of $J_k$. The semantics are not aligned, but this does not affect the proof of this case.


3. Uninterpreted parameters(case 2)

Wrong version: 
\begin{verbatim}
  Variable pairwise_task_interference :
    sporadic_task -> sporadic_task -> time -> time -> time.
\end{verbatim}    
Only the type expressing an object is modeled, but not its actual semantics.

4. the vacuous truth problem (case 3)

Wrong version: 
\begin{verbatim}
  Definition maximal_interference_job_of_task (tsk : sporadic_task) (j_star : Job) : Prop :=
    arrives_in arr_seq j_star /\
    job_task j_star = tsk /\
    forall j,
      arrives_in arr_seq j ->
      job_task j = tsk ->
      total_interference_of_job_window j <= total_interference_of_job_window j_star.
     Theorem Theorem6 :
    taskset_schedulable <->
    forall tsk,
      tsk \in ts ->
      forall j_star,
        maximal_interference_job_of_task tsk j_star ->
        theorem6_condition tsk j_star.   
\end{verbatim} 
It does not express existence, nor does it express the idea of 'first fix a worst‑case interference witness, and then check the condition on this witness'. If a certain task tsk does not have any jstar that satisfies maximal-interference-job-of-task, then for any jstar the antecedent is false, so the implication becomes vacuously true.

5. Missing precondition (case 4)
Wrong version: 
\begin{verbatim}
     Definition maximum_response_time_bounded_by (tsk : sporadic_task) (R : time) : Prop :=
      forall R_actual,
        is_maximum_response_time_of_task tsk R_actual ->
        R_actual <= R.   
\end{verbatim} 
It relies on a definition of ``task's maximum response time'' that takes the maximum over all $j$ with $\operatorname{job\_task}(j) = \mathtt{tsk}$, but there is no arrival sequence, no schedule/completion semantics, and not even a restriction that these $j$ must be jobs that actually arrive in the system. Semantically, it is not bound to be ``an upper bound on the maximum response time of task $\tau_k$ in the analyzed system''.

6. An implicit assumption is missing (case 5)

Wrong version: 
\begin{verbatim}
     Theorem RTSS2007_Theorem3 :
    forall tsk j_star R_ub,
      arrives_in arr_seq j_star ->
      job_task j_star = tsk ->
      is_maximum_response_time_witness tsk j_star ->
      \sum_(tsk_other <- other_tasks tsk)
        minn
          (task_interference job_arrival job_cost job_task sched j_star tsk_other
                             (job_arrival j_star) (job_arrival j_star + R_ub))
          (R_ub - task_cost tsk + 1)
      < num_cpus * (R_ub - task_cost tsk + 1) ->
      is_response_time_bound_of_task job_arrival job_cost job_task arr_seq sched tsk R_ub.
\end{verbatim} 
Correct version:
\begin{verbatim}
  add assumption R_ub >= task_cost tsk
\end{verbatim}
Although not explicitly stated in the paper, there is an obvious and conventional prerequisite for this theorem to hold: the response time must be at least the task's cost. The erroneous modeling omits this prerequisite.

(case 7)
Wrong version: 
\begin{verbatim}
  Theorem bertogna_cirinei_theorem4 :
      workload analyzed_task a b <=
      theorem4_workload_bound analyzed_task (b - a).
\end{verbatim} 
The analysis interval in the paper is \([a, b)\), which implicitly assumes the condition \(a < b\), but this is not reflected in the modeling.

7. Semantic incompleteness
Wrong version: 
\begin{verbatim}
  TVariable t0 : time.


      Definition all_processors_busy_with_higher_priority_work :=
        forall t cpu,
          t0 <= t < job_arrival j ->
          exists j_hp,
            scheduled_on sched j_hp cpu t /\
            higher_eq_priority (job_task j_hp) tsk.
\end{verbatim} 
$t_0$ is the start of the earliest busy period, but this modeling only expresses part of the conditions for $t_0$: the processor is busy from $t_0$ to $r_k$, and it does not express that it is the earliest start.

Wrong version: (case 15)
\begin{verbatim}
  (* Section IV-A introduces the extended busy-period start t0. *)
    Variable t0: time.

    (* By definition of the extended busy period, t0 precedes the analyzed release. *)
    Hypothesis H_t0_before_release:
      t0 <= job_arrival analyzed_job.

    (* The paper defines t0 so that all processors execute higher-priority work before rk. *)
    Hypothesis H_all_cpus_busy_with_higher_priority_tasks:
      forall t cpu,
        t0 <= t ->
        t < job_arrival analyzed_job ->
          exists j_hp,
          sched cpu t = Some j_hp /\
          higher_priority_task higher_eq_priority analyzed_task (job_task j_hp).
\end{verbatim} 
The semantics of binding the carry‑in task to higher‑priority tasks are missing. The paper has an implicit condition: the carry‑in task must be a higher‑priority task

8. additional assumptions introduced by the data type
(case 16)
\begin{verbatim}
Lemma lemma3 :
      forall x,
        before_end_of_busy_period x ->
        omega_k x %/ num_cpus > x - task_cost tsk_k.
\end{verbatim} 
In paper:

\textbf{Lemma 3.} For job \( J_k \) and all \( x < f_k - t_0 \), the following holds:
\[
\lfloor \frac{\Omega_k(x)}{M} \rfloor > x - C_k
\]
In this modeling, $x$ is modeled as a variable of type $\texttt{nat}$ in Coq, where subtraction on $\texttt{nat}$ does not yield negative numbers but truncates to $0$. Therefore, under this data type modeling, the premise $x > C_k$ needs to be added; otherwise, a counterexample $0 < 0$ would occur.


\subsection{Experiments on Formalization}


In this section we evaluate the capability of ProsaBuddy's formalizer. The goal is to understand to what extend ProsaBuddy can help with formalizing the lemma. Our experiments are conducted on 22 \guan{??}
lemmas.






Experiment Setting:

\begin{itemize}
    \item Experimental Task: For each benchmark instance, the input to the model consists of three sources: the PDF of the target paper, the PROSA library, and the skill files that provide task-specific modeling guidance. Given these materials, the model is required to generate a complete Coq modeling file for one target theorem from the paper. The expected output is not a partial snippet or a natural-language summary, but a self-contained theorem-level modeling artifact that captures the system context, the theorem-specific assumptions, the paper-specific intermediate definitions, and the final theorem statement within the Coq/PROSA setting.  \guan{how to specify which lemma to be formalized in that paper?}

   
    \item Benchmark: Casestudy except 8 and 10
    

    \item Prompting and Generation Protocol
     Prompt:
    1. Fill in the Coq `.v` file and ensure that the final file compiles with Coq.
   - The proof of the target theorem/lemma may be skipped with `Admitted.`
   - The file must still be syntactically and semantically valid.
   - All imports, sections, variables, definitions, hypotheses, and theorem statements must be well-scoped.

    2. \guan{is everything here by prompt?}. 
    Read only the paper content up to and including the target theorem/lemma.
   - Do not use definitions, assumptions, explanations, or results that appear after the target theorem/lemma 
   - The modeling must be based on the paper content before the target result and on the target theorem/lemma statement itself.
   - Be rigorous and comprehensive.
   - Even if a definition or assumption introduced before the target theorem/lemma does not seem useful for proving or stating the target theorem, it should still be modeled if it is part of the paper’s model.

    3. Follow the modeling style of the Prosa library.
   - Use `Section`s to organize parameters, assumptions, definitions, and results.
   - Carefully distinguish between `Variable`, `Definition`, and `Hypothesis`.
   - Prefer existing Prosa concepts, structures, and naming conventions whenever appropriate.
   - Do not unnecessarily redefine concepts that already exist in Prosa.

   Detailed workflow:

Step 1: Select Prosa imports, variables, and hypotheses.
Step 2: Model paper-specific definitions and assumptions not already present in Prosa.
Step 3: Model the target theorem/lemma.

Generation Budget ?

Retry Policy?

Randomness Control?
\item Evaluation Protocol
Level 1: Selection of PROSA Variables and Hypotheses.
Level 1 evaluates whether the model correctly identifies and introduces the reusable Variables and Hypothesises that can be taken from the PROSA library. For each case study, we first construct a human reference set of PROSA-aligned variables and hypotheses that are judged necessary to model the paper up to the target theorem. The Level 1 score is then computed as the ratio between the number of correctly selected items produced by the model and the number of items in the human reference set. If the model introduces incorrect or unjustified hypotheses, these are explicitly marked in the evaluation results. Importantly, if a hypothesis or modeling assumption could have been directly reused from PROSA but is instead reconstructed by the model itself, it is still counted as correct as long as the reconstructed version is semantically correct.

Level 2: Modeling of Paper-Specific Concepts Beyond PROSA.
Level 2 evaluates the modeling of concepts that are required by the paper but are not already available in PROSA. For each target case, we identify the set of paper-specific concepts that must be modeled before the theorem can be stated faithfully. Each concept is scored using a three-level rubric. A concept receives 1 point if its semantics are fully correct. It receives 0.5 points if it is partially correct, meaning that the core semantics are correct but incomplete, for example because important boundary conditions, minimality, existence conditions, legality constraints, or part of the essential relation are missing, even though the concept is attached to the correct mathematical object. It receives 0 points if it is only represented by a name, a variable, a comment, or a weak assumption without checkable semantics, or if it is absent, seriously misdirected, attached to the wrong object, or expressed by a fundamentally incorrect formula. The final Level 2 score for a case study is the average score across all required paper-specific concepts in that case.

Level 3: Modeling of the Target Theorem.
Level 3 evaluates the formalization of the target theorem statement itself. This level focuses on whether the generated theorem faithfully captures the mathematical meaning of the result in the paper. We again use a three-level rubric. A theorem receives 1 point if its semantics are fully correct: the target conclusion is correct, the necessary assumptions are essentially correct, and the logical structure, including quantifiers and implication directions, matches the intended theorem. It receives 0.5 points if it is partially correct: the statement captures the main idea of the theorem but omits some assumptions, weakens the conclusion, leaves boundary conditions imprecise, or relies on incorrectly modeled definitions. It receives 0 points if the theorem is completely incorrect or substantially departs from the intended meaning of the original result.


\end{itemize}


Experiment Results:

 \begin{table*}[htbp]
  \centering
  \caption{Task1-Our-Method} % 表格标题（可修改）
  \tiny % 字体大小适配20列，避免溢出（可改为tiny/normal）
  \setlength{\tabcolsep}{3pt} % 调整列间距，确保表格完整显示
  \begin{tabular}{@{}cccccccccccccccccccccccccc@{}} % 20个c表示20列居中对齐
    \toprule % 顶部粗线 
         & case1 & case2 & case3 & case4 & case5 & case6 & case7 &  case9 &
    case11 & case12 & case13 & case14 & case15 & case16& case17 & case18 & case19 & case20 & case21& case22& case23& case24 & avg \\
    \midrule 
  level 1 &92.6\% & 68.9\%/100\% & 92.3\% & 87.1\% & 100\% & 92.9\% & 96.2\%-1 & 100\% & 93.5\% & 100\% & 78.1\%/84.4 & 76.7\% & 81.3\% & 84.4\% & 97.0\% & 70.6\% & 83.3\% & 80.0\% & 80\% &63.3\%+1& 67.3\%+2 &80.5\% &85.3\% \\
  
 level 2 & 1 & 1/0,5 & 0.88 & 1 & / & 0 & 1 & 0.7 & 0.94 & 0.63 & 0.91/0.73 &? & 0.71 & 0.71 & 0.83 & 0.94 &1 & 0.9 & 1 & 0.8/1 & 0.94 & 1 &0.85\\
     level 3 & 1 & 1 & 1 & 0.5 &0.5 & 0.5 & 0.5/1 & 1 & 1 & 1 & 0.5/1 & ? & 1 & 0.5 & 1 & 1 & 1 & 1 & 1 & 1 &1 &1 &0.88\\
    \bottomrule % 底部粗线
  \end{tabular}
\end{table*}

 \begin{table*}[htbp]
  \centering
  \caption{Task1-Opencode} % 表格标题（可修改）
  \tiny % 字体大小适配20列，避免溢出（可改为tiny/normal）
  \setlength{\tabcolsep}{3pt} % 调整列间距，确保表格完整显示
  \begin{tabular}{@{}cccccccccccccccccccccccccc@{}} % 20个c表示20列居中对齐
    \toprule % 顶部粗线 
         & case1 & case2 & case3 & case4 & case5 & case6 & case7 &  case9 &
    case11 & case12 & case13 & case14 & case15 & case16& case17 & case18 & case19 & case20 & case21& case22& case23& case24& avg \\
    \midrule 
  level 1 & 88.9\% &81.5\%&96.2\% &45.2\%&100\%& 92.9\%&80.1\%&90.0\%& 87.1\%-o& 67.1\%&81.3\%-o &76.7\%&59.4\%&93.8\%-o&87.5\%&65.7\%&83.3\%&64.7\% &74.3\%&24.2\%&25.7\%&78.0\%&74.7\%\\
  
 level 2& 0.5&0& 0.63&0.5&/& 0&0.5& 0.6 & 0.56 &0.38&0.59&0.29& 0.29& 0.43&0.67&0.61&0.875&0.7&0.79&1&0.75&1&0.53\\
     level 3&  1&0.5&1&0.5&1& 0.5&1 & 1& 0.5& 0.5&0.5&0&0.5&0.5&1&0.5&1&0.5&1&1&0.5&1 &0.70\\
    \bottomrule % 底部粗线
  \end{tabular}
\end{table*}




\subsection{Task Definition}
\label{subsec:task}

Given (1) a paper PDF, (2) an existing Coq development in \texttt{.v} files, and (3) optionally a curated assumption bank ( from Prosa), the task is to complete the assumptions required by the formalization.

The output of the system consists of:
\begin{enumerate}
    \item a revised \texttt{.v} file with added assumptions;
    \item a structured justification report for each adopted assumption, including evidence and source attribution;
    \item generation-time statistics for each instance.
\end{enumerate}



\guan{move this part to the methodology part; what to say to justify this? rename the last category}
We distinguish three categories of assumptions:
\begin{itemize}
    \item \textbf{Model assumptions}: assumptions about the task model, scheduler semantics, timing semantics, workload semantics, etc.
    \item \textbf{Data-structure assumptions}: assumptions about records, functions, mappings, domains, well-formedness conditions, and representation invariants required by the Coq development.
    \item \textbf{Proof-related assumptions}: assumptions used specifically to support proof reasoning, such as first-missed-deadline arguments, maximal busy intervals, or technical side conditions required by intermediate lemmas.
\end{itemize}


We consider two generation settings.
\begin{itemize}
    \item \textbf{Generate-only}: the LLM generates assumptions directly from the paper and the current Coq artifact.
    \item \textbf{Hybrid}: the LLM is additionally given an assumption bank and is instructed to first select suitable assumptions from the bank, and only add new ones when the bank is insufficient.
\end{itemize}

\guan{who is the baseline we compare with? opencode; academic SOTA?? (to check and confirm)}


\guan{
\begin{itemize}
    \item Proving agent
        \begin{itemize}
            \item $t_0$,  
            \item the auxiliary definitions needed by the proof: 
            example: carry-in carry-out; TODO: find more cases 
            
        \end{itemize}
    \item Formalization agent
        \begin{itemize}
            \item select (not generate) assumptions; assumption classification;

                          
            \item Problem 1: the definition data type problem: we want to reuse the PROSA's definitions and related lemma, so make make sure the data type consistency. LLM sometimes will use them with other data types, inconsistent.
            \begin{itemize}
            \item  example: task, use a data type inconsistent with PROSA
            \end{itemize}
            Solution: we should give a list to explain the data type of all the definitions; 
            TODO: can we write a script to automatically check the data type consistency?



            \item Problem 2: some new complex definition, LLM cannot understand it by only reading the paper.
            \begin{itemize}
                \item  example: $t_0$
            \end{itemize}     
            Current Solution: human manually add it? 
            TODO: improve the agent design

            \item how the human confirm the correctness of the generated formalization


            \item note the difference between "basic/type" definition in prosa and the "concept" definition in the paper
            
            \item human confirm; $90\%$ precision
        \end{itemize}
\end{itemize}
}
